# Supplementary material for: Dreaming in Distribution: Understanding the Out-of-Distribution Capabilities of Video Generation Models
Source: arXiv:2611.38491 source file (2026-11-28)
Supplement: Supplementary file 1 [file supp_labels.tex]

% Auto-generated from supp.aux for standalone main-paper compilation (e.g., arXiv AutoTeX).
\makeatletter
\global\@namedef{r@app:notation}{{A}{S2}{}{}{}}
\global\@namedef{r@app:notation@cref}{{[section][1][]A}{[S1][2][]S2}{}{}{}}
\global\@namedef{r@tab:notation}{{S1}{S3}{}{}{}}
\global\@namedef{r@tab:notation@cref}{{[table][1][]S1}{[S1][3][]S3}{}{}{}}
\global\@namedef{r@app:related}{{B}{S5}{}{}{}}
\global\@namedef{r@app:related@cref}{{[section][2][]B}{[S1][5][]S5}{}{}{}}
\global\@namedef{r@fig:five-overview}{{S1}{S5}{}{}{}}
\global\@namedef{r@fig:five-overview@cref}{{[figure][1][]S1}{[S1][5][]S5}{}{}{}}
\global\@namedef{r@app:related-datasets}{{B.1}{S6}{}{}{}}
\global\@namedef{r@app:related-datasets@cref}{{[subsection][1][2]B.1}{[S1][6][]S6}{}{}{}}
\global\@namedef{r@app:related-tables}{{B.1}{S6}{}{}{}}
\global\@namedef{r@app:related-tables@cref}{{[subsection][1][2]B.1}{[S1][6][]S6}{}{}{}}
\global\@namedef{r@fig:five-tasks}{{S2}{S7}{}{}{}}
\global\@namedef{r@fig:five-tasks@cref}{{[figure][2][]S2}{[S1][6][]S7}{}{}{}}
\global\@namedef{r@tab:dataset_landscape}{{S2}{S7}{}{}{}}
\global\@namedef{r@tab:dataset_landscape@cref}{{[table][2][]S2}{[S1][6][]S7}{}{}{}}
\global\@namedef{r@app:related-long}{{B.2}{S8}{}{}{}}
\global\@namedef{r@app:related-long@cref}{{[subsection][2][2]B.2}{[S1][8][]S8}{}{}{}}
\global\@namedef{r@tab:longvideo_landscape}{{S3}{S8}{}{}{}}
\global\@namedef{r@tab:longvideo_landscape@cref}{{[table][3][]S3}{[S1][8][]S8}{}{}{}}
\global\@namedef{r@tab:vdm_landscape}{{S4}{S9}{}{}{}}
\global\@namedef{r@tab:vdm_landscape@cref}{{[table][4][]S4}{[S1][9][]S9}{}{}{}}
\global\@namedef{r@app:related-antic}{{B.3}{S10}{}{}{}}
\global\@namedef{r@app:related-antic@cref}{{[subsection][3][2]B.3}{[S1][10][]S10}{}{}{}}
\global\@namedef{r@tab:mllm_landscape}{{S5}{S10}{}{}{}}
\global\@namedef{r@tab:mllm_landscape@cref}{{[table][5][]S5}{[S1][10][]S10}{}{}{}}
\global\@namedef{r@app:related-reward}{{B.4}{S11}{}{}{}}
\global\@namedef{r@app:related-reward@cref}{{[subsection][4][2]B.4}{[S1][11][]S11}{}{}{}}
\global\@namedef{r@tab:videval_landscape}{{S6}{S11}{}{}{}}
\global\@namedef{r@tab:videval_landscape@cref}{{[table][6][]S6}{[S1][11][]S11}{}{}{}}
\global\@namedef{r@app:dataset}{{C}{S12}{}{}{}}
\global\@namedef{r@app:dataset@cref}{{[section][3][]C}{[S1][12][]S12}{}{}{}}
\global\@namedef{r@app:dataset-stats}{{C}{S12}{}{}{}}
\global\@namedef{r@app:dataset-stats@cref}{{[section][3][]C}{[S1][12][]S12}{}{}{}}
\global\@namedef{r@app:pnr-annotation}{{C.1}{S12}{}{}{}}
\global\@namedef{r@app:pnr-annotation@cref}{{[subsection][1][3]C.1}{[S1][12][]S12}{}{}{}}
\global\@namedef{r@eq:segment-stats}{{S1}{S12}{}{}{}}
\global\@namedef{r@eq:segment-stats@cref}{{[equation][1][]S1}{[S1][12][]S12}{}{}{}}
\global\@namedef{r@fig:pnr-tool}{{S3}{S13}{}{}{}}
\global\@namedef{r@fig:pnr-tool@cref}{{[figure][3][]S3}{[S1][12][]S13}{}{}{}}
\global\@namedef{r@tab:dataset-stats}{{S7}{S13}{}{}{}}
\global\@namedef{r@tab:dataset-stats@cref}{{[table][7][]S7}{[S1][12][]S13}{}{}{}}
\global\@namedef{r@fig:dataset-stats}{{S4}{S13}{}{}{}}
\global\@namedef{r@fig:dataset-stats@cref}{{[figure][4][]S4}{[S1][12][]S13}{}{}{}}
\global\@namedef{r@app:curation-subsets}{{C.2}{S13}{}{}{}}
\global\@namedef{r@app:curation-subsets@cref}{{[subsection][2][3]C.2}{[S1][13][]S13}{}{}{}}
\global\@namedef{r@tab:cohort-provenance}{{S8}{S14}{}{}{}}
\global\@namedef{r@tab:cohort-provenance@cref}{{[table][8][]S8}{[S1][14][]S14}{}{}{}}
\global\@namedef{r@app:evalset}{{D}{S14}{}{}{}}
\global\@namedef{r@app:evalset@cref}{{[section][4][]D}{[S1][14][]S14}{}{}{}}
\global\@namedef{r@app:review-form}{{D.1}{S14}{}{}{}}
\global\@namedef{r@app:review-form@cref}{{[subsection][1][4]D.1}{[S1][14][]S14}{}{}{}}
\global\@namedef{r@fig:review-grid}{{S5a}{S15}{}{}{}}
\global\@namedef{r@fig:review-grid@cref}{{[subfigure][1][5]S5a}{[S1][14][]S15}{}{}{}}
\global\@namedef{r@sub@fig:review-grid}{{a}{S15}{}{}{}}
\global\@namedef{r@sub@fig:review-grid@cref}{{[subfigure][1][5]S5a}{[S1][14][]S15}{}{}{}}
\global\@namedef{r@fig:review-studio}{{S5b}{S15}{}{}{}}
\global\@namedef{r@fig:review-studio@cref}{{[subfigure][2][5]S5b}{[S1][14][]S15}{}{}{}}
\global\@namedef{r@sub@fig:review-studio}{{b}{S15}{}{}{}}
\global\@namedef{r@sub@fig:review-studio@cref}{{[subfigure][2][5]S5b}{[S1][14][]S15}{}{}{}}
\global\@namedef{r@fig:review-screens}{{S5}{S15}{}{}{}}
\global\@namedef{r@fig:review-screens@cref}{{[figure][5][]S5}{[S1][14][]S15}{}{}{}}
\global\@namedef{r@app:alignment-metric}{{D.2}{S15}{}{}{}}
\global\@namedef{r@app:alignment-metric@cref}{{[subsection][2][4]D.2}{[S1][15][]S15}{}{}{}}
\global\@namedef{r@fig:arch-judge}{{S6}{S16}{}{}{}}
\global\@namedef{r@fig:arch-judge@cref}{{[figure][6][]S6}{[S1][16][]S16}{}{}{}}
\global\@namedef{r@fig:five-judge}{{S7}{S17}{}{}{}}
\global\@namedef{r@fig:five-judge@cref}{{[figure][7][]S7}{[S1][17][]S17}{}{}{}}
\global\@namedef{r@fig:ten-segment-grid}{{S7}{S17}{}{}{}}
\global\@namedef{r@fig:ten-segment-grid@cref}{{[figure][7][]S7}{[S1][17][]S17}{}{}{}}
\global\@namedef{r@eq:kappa}{{S2}{S18}{}{}{}}
\global\@namedef{r@eq:kappa@cref}{{[equation][2][]S2}{[S1][17][]S18}{}{}{}}
\global\@namedef{r@app:mllms}{{E}{S18}{}{}{}}
\global\@namedef{r@app:mllms@cref}{{[section][5][]E}{[S1][18][]S18}{}{}{}}
\global\@namedef{r@app:gt-gemini}{{E.1}{S18}{}{}{}}
\global\@namedef{r@app:gt-gemini@cref}{{[subsection][1][5]E.1}{[S1][18][]S18}{}{}{}}
\global\@namedef{r@sec:gt_protocol}{{E.1}{S18}{}{}{}}
\global\@namedef{r@sec:gt_protocol@cref}{{[subsection][1][5]E.1}{[S1][18][]S18}{}{}{}}
\global\@namedef{r@app:gt-prompt}{{E.1.2}{S19}{}{}{}}
\global\@namedef{r@app:gt-prompt@cref}{{[subsubsection][2][5,1]E.1.2}{[S1][19][]S19}{}{}{}}
\global\@namedef{r@sec:mllm_anticipation}{{E.2}{S21}{}{}{}}
\global\@namedef{r@sec:mllm_anticipation@cref}{{[subsection][2][5]E.2}{[S1][21][]S21}{}{}{}}
\global\@namedef{r@fig:forecast-task}{{S8}{S21}{}{}{}}
\global\@namedef{r@fig:forecast-task@cref}{{[figure][8][]S8}{[S1][21][]S21}{}{}{}}
\global\@namedef{r@app:annotation}{{E.2.1}{S22}{}{}{}}
\global\@namedef{r@app:annotation@cref}{{[subsubsection][1][5,2]E.2.1}{[S1][21][]S22}{}{}{}}
\global\@namedef{r@sec:textual_schema}{{E.2.1}{S22}{}{}{}}
\global\@namedef{r@sec:textual_schema@cref}{{[subsubsection][1][5,2]E.2.1}{[S1][21][]S22}{}{}{}}
\global\@namedef{r@eq:schema}{{S3}{S22}{}{}{}}
\global\@namedef{r@eq:schema@cref}{{[equation][3][]S3}{[S1][21][]S22}{}{}{}}
\global\@namedef{r@sec:timestamp_spec}{{E.2.1}{S22}{}{}{}}
\global\@namedef{r@sec:timestamp_spec@cref}{{[subsubsection][1][5,2]E.2.1}{[S1][22][]S22}{}{}{}}
\global\@namedef{r@fig:five-grid}{{S9}{S22}{}{}{}}
\global\@namedef{r@fig:five-grid@cref}{{[figure][9][]S9}{[S1][22][]S22}{}{}{}}
\global\@namedef{r@app:video-understanding}{{E.2.2}{S23}{}{}{}}
\global\@namedef{r@app:video-understanding@cref}{{[subsubsection][2][5,2]E.2.2}{[S1][22][]S23}{}{}{}}
\global\@namedef{r@app:agentic-arch}{{E.2.2}{S23}{}{}{}}
\global\@namedef{r@app:agentic-arch@cref}{{[subsubsection][2][5,2]E.2.2}{[S1][22][]S23}{}{}{}}
\global\@namedef{r@fig:arch-anticipation}{{S10}{S23}{}{}{}}
\global\@namedef{r@fig:arch-anticipation@cref}{{[figure][10][]S10}{[S1][23][]S23}{}{}{}}
\global\@namedef{r@fig:early-detection}{{S11}{S24}{}{}{}}
\global\@namedef{r@fig:early-detection@cref}{{[figure][11][]S11}{[S1][24][]S24}{}{}{}}
\global\@namedef{r@eq:factorization}{{S4}{S25}{}{}{}}
\global\@namedef{r@eq:factorization@cref}{{[equation][4][]S4}{[S1][25][]S25}{}{}{}}
\global\@namedef{r@fig:five-cascade}{{S12}{S25}{}{}{}}
\global\@namedef{r@fig:five-cascade@cref}{{[figure][12][]S12}{[S1][25][]S25}{}{}{}}
\global\@namedef{r@alg:por}{{1}{S26}{}{}{}}
\global\@namedef{r@alg:por@cref}{{[algorithm][1][]1}{[S1][26][]S26}{}{}{}}
\global\@namedef{r@eq:conf}{{S5}{S26}{}{}{}}
\global\@namedef{r@eq:conf@cref}{{[equation][5][]S5}{[S1][26][]S26}{}{}{}}
\global\@namedef{r@eq:seqconf}{{S6}{S27}{}{}{}}
\global\@namedef{r@eq:seqconf@cref}{{[equation][6][]S6}{[S1][26][]S27}{}{}{}}
\global\@namedef{r@sec:mllm_evaluation}{{E.2.3}{S27}{}{}{}}
\global\@namedef{r@sec:mllm_evaluation@cref}{{[subsubsection][3][5,2]E.2.3}{[S1][27][]S27}{}{}{}}
\global\@namedef{r@eq:simprim}{{S7}{S27}{}{}{}}
\global\@namedef{r@eq:simprim@cref}{{[equation][7][]S7}{[S1][27][]S27}{}{}{}}
\global\@namedef{r@eq:tuplesim}{{S8}{S27}{}{}{}}
\global\@namedef{r@eq:tuplesim@cref}{{[equation][8][]S8}{[S1][27][]S27}{}{}{}}
\global\@namedef{r@eq:assign}{{S9}{S27}{}{}{}}
\global\@namedef{r@eq:assign@cref}{{[equation][9][]S9}{[S1][27][]S27}{}{}{}}
\global\@namedef{r@fig:five-tuples}{{S13}{S28}{}{}{}}
\global\@namedef{r@fig:five-tuples@cref}{{[figure][13][]S13}{[S1][27][]S28}{}{}{}}
\global\@namedef{r@eq:tripletsim}{{S10}{S28}{}{}{}}
\global\@namedef{r@eq:tripletsim@cref}{{[equation][10][]S10}{[S1][28][]S28}{}{}{}}
\global\@namedef{r@sec:results-antic}{{E.2.4}{S29}{}{}{}}
\global\@namedef{r@sec:results-antic@cref}{{[subsubsection][4][5,2]E.2.4}{[S1][29][]S29}{}{}{}}
\global\@namedef{r@sec:results-antic-rows}{{E.2.4}{S29}{}{}{}}
\global\@namedef{r@sec:results-antic-rows@cref}{{[subsubsection][4][5,2]E.2.4}{[S1][29][]S29}{}{}{}}
\global\@namedef{r@sec:results-antic-cols}{{E.2.4}{S29}{}{}{}}
\global\@namedef{r@sec:results-antic-cols@cref}{{[subsubsection][4][5,2]E.2.4}{[S1][29][]S29}{}{}{}}
\global\@namedef{r@sec:results-antic-qwen}{{E.2.4}{S29}{}{}{}}
\global\@namedef{r@sec:results-antic-qwen@cref}{{[subsubsection][4][5,2]E.2.4}{[S1][29][]S29}{}{}{}}
\global\@namedef{r@sec:results-antic-gemini}{{E.2.4}{S29}{}{}{}}
\global\@namedef{r@sec:results-antic-gemini@cref}{{[subsubsection][4][5,2]E.2.4}{[S1][29][]S29}{}{}{}}
\global\@namedef{r@sec:results-antic-combined}{{E.2.4}{S29}{}{}{}}
\global\@namedef{r@sec:results-antic-combined@cref}{{[subsubsection][4][5,2]E.2.4}{[S1][29][]S29}{}{}{}}
\global\@namedef{r@app:antic-figures}{{E.2.4}{S29}{}{}{}}
\global\@namedef{r@app:antic-figures@cref}{{[subsubsection][4][5,2]E.2.4}{[S1][29][]S29}{}{}{}}
\global\@namedef{r@fig:antic-components}{{S14}{S30}{}{}{}}
\global\@namedef{r@fig:antic-components@cref}{{[figure][14][]S14}{[S1][29][]S30}{}{}{}}
\global\@namedef{r@app:agentic-eval}{{E.3}{S30}{}{}{}}
\global\@namedef{r@app:agentic-eval@cref}{{[subsection][3][5]E.3}{[S1][30][]S30}{}{}{}}
\global\@namedef{r@fig:antic-overall}{{S15}{S31}{}{}{}}
\global\@namedef{r@fig:antic-overall@cref}{{[figure][15][]S15}{[S1][29][]S31}{}{}{}}
\global\@namedef{r@fig:five-outcome}{{S16}{S31}{}{}{}}
\global\@namedef{r@fig:five-outcome@cref}{{[figure][16][]S16}{[S1][29][]S31}{}{}{}}
\global\@namedef{r@app:eval-motivation}{{E.3.1}{S31}{}{}{}}
\global\@namedef{r@app:eval-motivation@cref}{{[subsubsection][1][5,3]E.3.1}{[S1][31][]S31}{}{}{}}
\global\@namedef{r@fig:antic-qual}{{S17}{S32}{}{}{}}
\global\@namedef{r@fig:antic-qual@cref}{{[figure][17][]S17}{[S1][29][]S32}{}{}{}}
\global\@namedef{r@app:eval-base}{{E.3.2}{S32}{}{}{}}
\global\@namedef{r@app:eval-base@cref}{{[subsubsection][2][5,3]E.3.2}{[S1][32][]S32}{}{}{}}
\global\@namedef{r@app:eval-math}{{E.3.2}{S33}{}{}{}}
\global\@namedef{r@app:eval-math@cref}{{[subsubsection][2][5,3]E.3.2}{[S1][33][]S33}{}{}{}}
\global\@namedef{r@eq:check-mass}{{S11}{S33}{}{}{}}
\global\@namedef{r@eq:check-mass@cref}{{[equation][11][]S11}{[S1][33][]S33}{}{}{}}
\global\@namedef{r@fig:arch-evaluator-full}{{S18}{S34}{}{}{}}
\global\@namedef{r@fig:arch-evaluator-full@cref}{{[figure][18][]S18}{[S1][33][]S34}{}{}{}}
\global\@namedef{r@eq:check-score}{{S12}{S34}{}{}{}}
\global\@namedef{r@eq:check-score@cref}{{[equation][12][]S12}{[S1][33][]S34}{}{}{}}
\global\@namedef{r@eq:agent-interval}{{S13}{S35}{}{}{}}
\global\@namedef{r@eq:agent-interval@cref}{{[equation][13][]S13}{[S1][34][]S35}{}{}{}}
\global\@namedef{r@eq:verdict}{{S14}{S35}{}{}{}}
\global\@namedef{r@eq:verdict@cref}{{[equation][14][]S14}{[S1][35][]S35}{}{}{}}
\global\@namedef{r@eq:inquiry}{{S15}{S35}{}{}{}}
\global\@namedef{r@eq:inquiry@cref}{{[equation][15][]S15}{[S1][35][]S35}{}{}{}}
\global\@namedef{r@app:clip-audit}{{E.3.2}{S36}{}{}{}}
\global\@namedef{r@app:clip-audit@cref}{{[subsubsection][2][5,3]E.3.2}{[S1][35][]S36}{}{}{}}
\global\@namedef{r@fig:agentic-pro}{{S19}{S36}{}{}{}}
\global\@namedef{r@fig:agentic-pro@cref}{{[figure][19][]S19}{[S1][36][]S36}{}{}{}}
\global\@namedef{r@eq:pro-cost}{{S16}{S36}{}{}{}}
\global\@namedef{r@eq:pro-cost@cref}{{[equation][16][]S16}{[S1][36][]S36}{}{}{}}
\global\@namedef{r@app:legacy-tools}{{E.3.2}{S37}{}{}{}}
\global\@namedef{r@app:legacy-tools@cref}{{[subsubsection][2][5,3]E.3.2}{[S1][37][]S37}{}{}{}}
\global\@namedef{r@fig:arch-legacy}{{S20}{S37}{}{}{}}
\global\@namedef{r@fig:arch-legacy@cref}{{[figure][20][]S20}{[S1][37][]S37}{}{}{}}
\global\@namedef{r@fig:five-objects}{{S21}{S38}{}{}{}}
\global\@namedef{r@fig:five-objects@cref}{{[figure][21][]S21}{[S1][37][]S38}{}{}{}}
\global\@namedef{r@eq:track-sim}{{S17}{S39}{}{}{}}
\global\@namedef{r@eq:track-sim@cref}{{[equation][17][]S17}{[S1][39][]S39}{}{}{}}
\global\@namedef{r@app:mllm-judges}{{E.3.3}{S39}{}{}{}}
\global\@namedef{r@app:mllm-judges@cref}{{[subsubsection][3][5,3]E.3.3}{[S1][39][]S39}{}{}{}}
\global\@namedef{r@app:ft-math}{{E.3.3}{S39}{}{}{}}
\global\@namedef{r@app:ft-math@cref}{{[subsubsection][3][5,3]E.3.3}{[S1][39][]S39}{}{}{}}
\global\@namedef{r@eq:lora}{{S18}{S39}{}{}{}}
\global\@namedef{r@eq:lora@cref}{{[equation][18][]S18}{[S1][39][]S39}{}{}{}}
\global\@namedef{r@eq:sft}{{S19}{S40}{}{}{}}
\global\@namedef{r@eq:sft@cref}{{[equation][19][]S19}{[S1][39][]S40}{}{}{}}
\global\@namedef{r@eq:grpo-loss}{{S20}{S40}{}{}{}}
\global\@namedef{r@eq:grpo-loss@cref}{{[equation][20][]S20}{[S1][40][]S40}{}{}{}}
\global\@namedef{r@eq:reward}{{S21}{S40}{}{}{}}
\global\@namedef{r@eq:reward@cref}{{[equation][21][]S21}{[S1][40][]S40}{}{}{}}
\global\@namedef{r@eq:reward-terms}{{S22}{S40}{}{}{}}
\global\@namedef{r@eq:reward-terms@cref}{{[equation][22][]S22}{[S1][40][]S40}{}{}{}}
\global\@namedef{r@eq:verdict-tilt}{{S23}{S40}{}{}{}}
\global\@namedef{r@eq:verdict-tilt@cref}{{[equation][23][]S23}{[S1][40][]S40}{}{}{}}
\global\@namedef{r@app:ft-examples}{{E.3.3}{S41}{}{}{}}
\global\@namedef{r@app:ft-examples@cref}{{[subsubsection][3][5,3]E.3.3}{[S1][41][]S41}{}{}{}}
\global\@namedef{r@tab:ft-tasks}{{S9}{S41}{}{}{}}
\global\@namedef{r@tab:ft-tasks@cref}{{[table][9][]S9}{[S1][41][]S41}{}{}{}}
\global\@namedef{r@tab:physion-ft}{{S10}{S42}{}{}{}}
\global\@namedef{r@tab:physion-ft@cref}{{[table][10][]S10}{[S1][42][]S42}{}{}{}}
\global\@namedef{r@fig:judge-grid}{{S22}{S43}{}{}{}}
\global\@namedef{r@fig:judge-grid@cref}{{[figure][22][]S22}{[S1][42][]S43}{}{}{}}
\global\@namedef{r@fig:physion-ft}{{S23}{S43}{}{}{}}
\global\@namedef{r@fig:physion-ft@cref}{{[figure][23][]S23}{[S1][42][]S43}{}{}{}}
\global\@namedef{r@app:human}{{E.3.4}{S44}{}{}{}}
\global\@namedef{r@app:human@cref}{{[subsubsection][4][5,3]E.3.4}{[S1][44][]S44}{}{}{}}
\global\@namedef{r@fig:five-coverage}{{S24}{S44}{}{}{}}
\global\@namedef{r@fig:five-coverage@cref}{{[figure][24][]S24}{[S1][44][]S44}{}{}{}}
\global\@namedef{r@tab:judge-human-full}{{S11}{S45}{}{}{}}
\global\@namedef{r@tab:judge-human-full@cref}{{[table][11][]S11}{[S1][44][]S45}{}{}{}}
\global\@namedef{r@tab:human-group-a-full}{{S12}{S46}{}{}{}}
\global\@namedef{r@tab:human-group-a-full@cref}{{[table][12][]S12}{[S1][45][]S46}{}{}{}}
\global\@namedef{r@tab:judge-group-a-full}{{S13}{S46}{}{}{}}
\global\@namedef{r@tab:judge-group-a-full@cref}{{[table][13][]S13}{[S1][45][]S46}{}{}{}}
\global\@namedef{r@fig:judge-group-a}{{S25}{S46}{}{}{}}
\global\@namedef{r@fig:judge-group-a@cref}{{[figure][25][]S25}{[S1][45][]S46}{}{}{}}
\global\@namedef{r@tab:judge-group-b}{{S14}{S47}{}{}{}}
\global\@namedef{r@tab:judge-group-b@cref}{{[table][14][]S14}{[S1][47][]S47}{}{}{}}
\global\@namedef{r@tab:alignment-plan}{{S15}{S47}{}{}{}}
\global\@namedef{r@tab:alignment-plan@cref}{{[table][15][]S15}{[S1][47][]S47}{}{}{}}
\global\@namedef{r@fig:judge-cond-cosmos3}{{S26}{S48}{}{}{}}
\global\@namedef{r@fig:judge-cond-cosmos3@cref}{{[figure][26][]S26}{[S1][47][]S48}{}{}{}}
\global\@namedef{r@app:fixed-scores}{{E.3.5}{S48}{}{}{}}
\global\@namedef{r@app:fixed-scores@cref}{{[subsubsection][5][5,3]E.3.5}{[S1][48][]S48}{}{}{}}
\global\@namedef{r@fig:axes}{{S27}{S49}{}{}{}}
\global\@namedef{r@fig:axes@cref}{{[figure][27][]S27}{[S1][48][]S49}{}{}{}}
\global\@namedef{r@tab:axes}{{S16}{S49}{}{}{}}
\global\@namedef{r@tab:axes@cref}{{[table][16][]S16}{[S1][48][]S49}{}{}{}}
\global\@namedef{r@fig:five-scores}{{S28}{S50}{}{}{}}
\global\@namedef{r@fig:five-scores@cref}{{[figure][28][]S28}{[S1][48][]S50}{}{}{}}
\global\@namedef{r@eq:headlines}{{S24}{S51}{}{}{}}
\global\@namedef{r@eq:headlines@cref}{{[equation][24][]S24}{[S1][51][]S51}{}{}{}}
\global\@namedef{r@eq:horizon}{{S25}{S51}{}{}{}}
\global\@namedef{r@eq:horizon@cref}{{[equation][25][]S25}{[S1][51][]S51}{}{}{}}
\global\@namedef{r@app:anchoring}{{E.3.5}{S51}{}{}{}}
\global\@namedef{r@app:anchoring@cref}{{[subsubsection][5][5,3]E.3.5}{[S1][51][]S51}{}{}{}}
\global\@namedef{r@app:bt-model}{{E.3.5}{S52}{}{}{}}
\global\@namedef{r@app:bt-model@cref}{{[subsubsection][5][5,3]E.3.5}{[S1][52][]S52}{}{}{}}
\global\@namedef{r@eq:bt}{{S26}{S52}{}{}{}}
\global\@namedef{r@eq:bt@cref}{{[equation][26][]S26}{[S1][52][]S52}{}{}{}}
\global\@namedef{r@eq:bt-mm}{{S27}{S52}{}{}{}}
\global\@namedef{r@eq:bt-mm@cref}{{[equation][27][]S27}{[S1][52][]S52}{}{}{}}
\global\@namedef{r@app:plugins}{{F}{S53}{}{}{}}
\global\@namedef{r@app:plugins@cref}{{[section][6][]F}{[S1][52][]S53}{}{}{}}
\global\@namedef{r@fig:plugin-overview}{{S29}{S53}{}{}{}}
\global\@namedef{r@fig:plugin-overview@cref}{{[figure][29][]S29}{[S1][53][]S53}{}{}{}}
\global\@namedef{r@app:architectures}{{F.1}{S53}{}{}{}}
\global\@namedef{r@app:architectures@cref}{{[subsection][1][6]F.1}{[S1][53][]S53}{}{}{}}
\global\@namedef{r@app:wan-geometry}{{F.1.1}{S54}{}{}{}}
\global\@namedef{r@app:wan-geometry@cref}{{[subsubsection][1][6,1]F.1.1}{[S1][54][]S54}{}{}{}}
\global\@namedef{r@fig:arch-wan}{{S30}{S54}{}{}{}}
\global\@namedef{r@fig:arch-wan@cref}{{[figure][30][]S30}{[S1][54][]S54}{}{}{}}
\global\@namedef{r@eq:wan-chunks}{{S28}{S55}{}{}{}}
\global\@namedef{r@eq:wan-chunks@cref}{{[equation][28][]S28}{[S1][55][]S55}{}{}{}}
\global\@namedef{r@app:cosmos-geometry}{{F.1.2}{S56}{}{}{}}
\global\@namedef{r@app:cosmos-geometry@cref}{{[subsubsection][2][6,1]F.1.2}{[S1][56][]S56}{}{}{}}
\global\@namedef{r@fig:arch-cosmos}{{S31}{S56}{}{}{}}
\global\@namedef{r@fig:arch-cosmos@cref}{{[figure][31][]S31}{[S1][56][]S56}{}{}{}}
\global\@namedef{r@app:plugin-mechanisms}{{F.2}{S57}{}{}{}}
\global\@namedef{r@app:plugin-mechanisms@cref}{{[subsection][2][6]F.2}{[S1][57][]S57}{}{}{}}
\global\@namedef{r@app:plugin-prior}{{F.2.1}{S57}{}{}{}}
\global\@namedef{r@app:plugin-prior@cref}{{[subsubsection][1][6,2]F.2.1}{[S1][57][]S57}{}{}{}}
\global\@namedef{r@fig:plugin-tedio-bachvid}{{S32}{S58}{}{}{}}
\global\@namedef{r@fig:plugin-tedio-bachvid@cref}{{[figure][32][]S32}{[S1][57][]S58}{}{}{}}
\global\@namedef{r@fig:plugin-tedio}{{S32}{S58}{}{}{}}
\global\@namedef{r@fig:plugin-tedio@cref}{{[figure][32][]S32}{[S1][57][]S58}{}{}{}}
\global\@namedef{r@fig:plugin-bachvid}{{S32}{S58}{}{}{}}
\global\@namedef{r@fig:plugin-bachvid@cref}{{[figure][32][]S32}{[S1][57][]S58}{}{}{}}
\global\@namedef{r@eq:tedio-d}{{S29}{S58}{}{}{}}
\global\@namedef{r@eq:tedio-d@cref}{{[equation][29][]S29}{[S1][58][]S58}{}{}{}}
\global\@namedef{r@tab:prior-vs-ours}{{S17}{S59}{}{}{}}
\global\@namedef{r@tab:prior-vs-ours@cref}{{[table][17][]S17}{[S1][59][]S59}{}{}{}}
\global\@namedef{r@eq:bachvid}{{S30}{S60}{}{}{}}
\global\@namedef{r@eq:bachvid@cref}{{[equation][30][]S30}{[S1][60][]S60}{}{}{}}
\global\@namedef{r@app:memory}{{F.2.2}{S60}{}{}{}}
\global\@namedef{r@app:memory@cref}{{[subsubsection][2][6,2]F.2.2}{[S1][60][]S60}{}{}{}}
\global\@namedef{r@fig:plugin-memalign}{{S33}{S61}{}{}{}}
\global\@namedef{r@fig:plugin-memalign@cref}{{[figure][33][]S33}{[S1][60][]S61}{}{}{}}
\global\@namedef{r@eq:gate}{{S31}{S62}{}{}{}}
\global\@namedef{r@eq:gate@cref}{{[equation][31][]S31}{[S1][62][]S62}{}{}{}}
\global\@namedef{r@eq:memloss}{{S32}{S62}{}{}{}}
\global\@namedef{r@eq:memloss@cref}{{[equation][32][]S32}{[S1][62][]S62}{}{}{}}
\global\@namedef{r@tab:steer-hooks}{{S18}{S63}{}{}{}}
\global\@namedef{r@tab:steer-hooks@cref}{{[table][18][]S18}{[S1][63][]S63}{}{}{}}
\global\@namedef{r@app:plugin-results}{{F.3}{S63}{}{}{}}
\global\@namedef{r@app:plugin-results@cref}{{[subsection][3][6]F.3}{[S1][63][]S63}{}{}{}}
\global\@namedef{r@fig:plugin-qual}{{S34}{S64}{}{}{}}
\global\@namedef{r@fig:plugin-qual@cref}{{[figure][34][]S34}{[S1][63][]S64}{}{}{}}
\global\@namedef{r@app:activation}{{F.3.2}{S64}{}{}{}}
\global\@namedef{r@app:activation@cref}{{[subsubsection][2][6,3]F.3.2}{[S1][64][]S64}{}{}{}}
\global\@namedef{r@eq:noise-floor}{{S33}{S64}{}{}{}}
\global\@namedef{r@eq:noise-floor@cref}{{[equation][33][]S33}{[S1][64][]S64}{}{}{}}
\global\@namedef{r@app:full-results}{{F.3.3}{S65}{}{}{}}
\global\@namedef{r@app:full-results@cref}{{[subsubsection][3][6,3]F.3.3}{[S1][64][]S65}{}{}{}}
\global\@namedef{r@sec:results-rows}{{F.3.3}{S65}{}{}{}}
\global\@namedef{r@sec:results-rows@cref}{{[subsubsection][3][6,3]F.3.3}{[S1][64][]S65}{}{}{}}
\global\@namedef{r@fig:five-wan}{{S35}{S65}{}{}{}}
\global\@namedef{r@fig:five-wan@cref}{{[figure][35][]S35}{[S1][65][]S65}{}{}{}}
\global\@namedef{r@sec:results-columns}{{F.3.3}{S65}{}{}{}}
\global\@namedef{r@sec:results-columns@cref}{{[subsubsection][3][6,3]F.3.3}{[S1][65][]S65}{}{}{}}
\global\@namedef{r@sec:results-robust}{{F.3.3}{S65}{}{}{}}
\global\@namedef{r@sec:results-robust@cref}{{[subsubsection][3][6,3]F.3.3}{[S1][65][]S65}{}{}{}}
\global\@namedef{r@fig:plugin-stack}{{S36}{S66}{}{}{}}
\global\@namedef{r@fig:plugin-stack@cref}{{[figure][36][]S36}{[S1][65][]S66}{}{}{}}
\global\@namedef{r@app:judge-steering}{{F.3.4}{S66}{}{}{}}
\global\@namedef{r@app:judge-steering@cref}{{[subsubsection][4][6,3]F.3.4}{[S1][66][]S66}{}{}{}}
\global\@namedef{r@fig:judge-steering}{{S37}{S67}{}{}{}}
\global\@namedef{r@fig:judge-steering@cref}{{[figure][37][]S37}{[S1][66][]S67}{}{}{}}
\global\@namedef{r@app:conditioning}{{G}{S67}{}{}{}}
\global\@namedef{r@app:conditioning@cref}{{[section][7][]G}{[S1][67][]S67}{}{}{}}
\global\@namedef{r@app:cond-generation}{{G.1}{S67}{}{}{}}
\global\@namedef{r@app:cond-generation@cref}{{[subsection][1][7]G.1}{[S1][67][]S67}{}{}{}}
\global\@namedef{r@fig:cond-compiler}{{S38}{S68}{}{}{}}
\global\@namedef{r@fig:cond-compiler@cref}{{[figure][38][]S38}{[S1][67][]S68}{}{}{}}
\global\@namedef{r@app:cond-examples}{{G.2}{S69}{}{}{}}
\global\@namedef{r@app:cond-examples@cref}{{[subsection][2][7]G.2}{[S1][69][]S69}{}{}{}}
\global\@namedef{r@app:cond-performance}{{G.3}{S69}{}{}{}}
\global\@namedef{r@app:cond-performance@cref}{{[subsection][3][7]G.3}{[S1][69][]S69}{}{}{}}
\global\@namedef{r@app:cond-groups}{{G.3}{S69}{}{}{}}
\global\@namedef{r@app:cond-groups@cref}{{[subsection][3][7]G.3}{[S1][69][]S69}{}{}{}}
\global\@namedef{r@app:agentic-pilot}{{G.3.1}{S69}{}{}{}}
\global\@namedef{r@app:agentic-pilot@cref}{{[subsubsection][1][7,3]G.3.1}{[S1][69][]S69}{}{}{}}
\global\@namedef{r@fig:cond-text}{{S39}{S70}{}{}{}}
\global\@namedef{r@fig:cond-text@cref}{{[figure][39][]S39}{[S1][69][]S70}{}{}{}}
\global\@namedef{r@fig:agentic-qual}{{S40}{S71}{}{}{}}
\global\@namedef{r@fig:agentic-qual@cref}{{[figure][40][]S40}{[S1][69][]S71}{}{}{}}
\global\@namedef{r@app:cross-backbone}{{G.3.2}{S72}{}{}{}}
\global\@namedef{r@app:cross-backbone@cref}{{[subsubsection][2][7,3]G.3.2}{[S1][72][]S72}{}{}{}}
\global\@namedef{r@tab:cross-backbone-cond}{{S19}{S72}{}{}{}}
\global\@namedef{r@tab:cross-backbone-cond@cref}{{[table][19][]S19}{[S1][72][]S72}{}{}{}}
\global\@namedef{r@fig:bt-conditioning}{{S41}{S73}{}{}{}}
\global\@namedef{r@fig:bt-conditioning@cref}{{[figure][41][]S41}{[S1][72][]S73}{}{}{}}
\global\@namedef{r@app:paired-findings}{{G.3.3}{S73}{}{}{}}
\global\@namedef{r@app:paired-findings@cref}{{[subsubsection][3][7,3]G.3.3}{[S1][73][]S73}{}{}{}}
\global\@namedef{r@tab:closed-cc}{{S20}{S74}{}{}{}}
\global\@namedef{r@tab:closed-cc@cref}{{[table][20][]S20}{[S1][73][]S74}{}{}{}}
\global\@namedef{r@tab:cos-cond-oops}{{S21}{S74}{}{}{}}
\global\@namedef{r@tab:cos-cond-oops@cref}{{[table][21][]S21}{[S1][73][]S74}{}{}{}}
\global\@namedef{r@tab:paired-findings}{{S22}{S74}{}{}{}}
\global\@namedef{r@tab:paired-findings@cref}{{[table][22][]S22}{[S1][73][]S74}{}{}{}}
\global\@namedef{r@fig:five-allmodels}{{S42}{S75}{}{}{}}
\global\@namedef{r@fig:five-allmodels@cref}{{[figure][42][]S42}{[S1][73][]S75}{}{}{}}
\global\@namedef{r@app:tool-scores}{{G.4}{S75}{}{}{}}
\global\@namedef{r@app:tool-scores@cref}{{[subsection][4][7]G.4}{[S1][75][]S75}{}{}{}}
\global\@namedef{r@sec:results-tools}{{G.4}{S75}{}{}{}}
\global\@namedef{r@sec:results-tools@cref}{{[subsection][4][7]G.4}{[S1][75][]S75}{}{}{}}
\global\@namedef{r@tab:cond-wan-strict}{{S23}{S76}{}{}{}}
\global\@namedef{r@tab:cond-wan-strict@cref}{{[table][23][]S23}{[S1][75][]S76}{}{}{}}
\global\@namedef{r@tab:cond-wan-relaxed}{{S23}{S76}{}{}{}}
\global\@namedef{r@tab:cond-wan-relaxed@cref}{{[table][23][]S23}{[S1][75][]S76}{}{}{}}
\global\@namedef{r@fig:tools-group-a}{{S43}{S76}{}{}{}}
\global\@namedef{r@fig:tools-group-a@cref}{{[figure][43][]S43}{[S1][75][]S76}{}{}{}}
\global\@namedef{r@fig:tools-group-b}{{S44}{S77}{}{}{}}
\global\@namedef{r@fig:tools-group-b@cref}{{[figure][44][]S44}{[S1][75][]S77}{}{}{}}
\global\@namedef{r@app:pixverse-check}{{G.4}{S77}{}{}{}}
\global\@namedef{r@app:pixverse-check@cref}{{[subsection][4][7]G.4}{[S1][77][]S77}{}{}{}}
\global\@namedef{r@app:synthesis}{{H}{S78}{}{}{}}
\global\@namedef{r@app:synthesis@cref}{{[section][8][]H}{[S1][78][]S78}{}{}{}}
\global\@namedef{r@app:synthesis-findings}{{H.1}{S78}{}{}{}}
\global\@namedef{r@app:synthesis-findings@cref}{{[subsection][1][8]H.1}{[S1][78][]S78}{}{}{}}
\global\@namedef{r@tab:evidence-tiers}{{S24}{S79}{}{}{}}
\global\@namedef{r@tab:evidence-tiers@cref}{{[table][24][]S24}{[S1][79][]S79}{}{}{}}
\global\@namedef{r@app:synthesis-challenges}{{H.2}{S79}{}{}{}}
\global\@namedef{r@app:synthesis-challenges@cref}{{[subsection][2][8]H.2}{[S1][79][]S79}{}{}{}}
\global\@namedef{r@app:synthesis-limitations}{{H.3}{S80}{}{}{}}
\global\@namedef{r@app:synthesis-limitations@cref}{{[subsection][3][8]H.3}{[S1][79][]S80}{}{}{}}
\makeatother
